# Supplementary material for: Beating Backdoor Attack at Its Own Game
Source: arXiv:2307.15539 source file (2025-04-05)
Supplement: Supplementary file 1 [file appendix.tex]

\begin{algorithm}[t]
    \caption{Non-Adversarial Backdoor}
    \label{algo1}
    \begin{algorithmic}[1]
        \REQUIRE $\mathcal{D}_p=\{(\bm{x}_i, y_i)\}_{i=1}^N$ released by the attacker
        \STATE $\mathcal{D}_s', \mathcal{D}_c' \leftarrow \text{BACKDOOR-DETECTION}(\mathcal{D}_p, \mu)$
        \STATE $\mathcal{D}_p' \leftarrow \mathcal{D}_c'$
        \FORALL{$(\bm{x}, y)\in\mathcal{D}_s'$}
            \IF{$r(\bm{x}) \neq y$}
                \STATE $\mathcal{D}_p'\leftarrow \mathcal{D}_p'\cup \{(\mathcal{S}(\bm{x}), r(\bm{x}))\}$ 
            \ELSE
                \STATE $\mathcal{D}_p'\leftarrow \mathcal{D}_p'\cup \{(\bm{x}, y)\}$
            \ENDIF
        \ENDFOR
        \RETURN $\mathcal{D}_p'$
    \end{algorithmic}
\end{algorithm}

\section{Implementation Details}
\subsection{Metrics}
% We adopt two widely used metrics for the main results: attack success rate (ASR, ratio of poisoned samples mistakenly classified to the target class) and Clean Accuracy (CA, ratio of correctly predicted clean samples). 
% To test the effectiveness of our data filtering method, we further introduce backdoor accuracy (BA, ratio of correctly predicted backdoor samples), ratio of rejected clean data (C-REJ), prediction success rate (PSR, ratio of correctly predicted \textit{and not} rejected clean samples), ratio of rejected poisoned data (B-REJ), and defense success rate (DSR, ratio of correctly predicted \textit{or} rejected poisoned samples)
Let $\mathcal{D}_{test}=\{(\bm{x}, y)\}_{i=1}^n$ be a set of clean samples. 
$y_t$ is the attacker's target class. 
For simplicity, we denote $|\{ (\bm{x}, y)\in \mathcal{D}_{test} | condition \}|$ as $\text{\#}(condition)$. We compute the metrics following:
\begin{itemize}
    \item \textbf{ASR}: $\text{\#}({f_\theta(\mathcal{P}(\bm{x}))=y_t}\land y\neq y_t) / \text{\#}(y\neq y_t)$
    \item \textbf{CA}: $\text{\#}(f_\theta(\bm{x})=y) / \text{\#}(True)$
    \item \textbf{BA}: $\text{\#}(f_\theta(\mathcal{P}(\bm{x}))=y) / \text{\#}(True)$
\end{itemize}
The metrics below are utilized to evaluate NAB augmented with data filtering:
\begin{itemize}
    \item \textbf{C-REJ}: $\text{\#}(f_\theta(\mathcal{S}(\bm{x}))\neq f_\theta(\bm{x})) / \text{\#}(True)$
    \item \textbf{PSR}: $\text{\#}(f_\theta(\mathcal{S}(\bm{x})) = y \land f_\theta(\mathcal{S}(\bm{x}))= f_\theta(\bm{x})) / \text{\#}(True)$
    \item \textbf{B-REJ}: $\text{\#}(f_\theta(\mathcal{S}(\mathcal{P}(\bm{x})))\neq f_\theta(\mathcal{P}(\bm{x}))) / \text{\#}(True)$
    \item \textbf{DSR}: $\text{\#}( f_\theta(\mathcal{S}(\mathcal{P}(\bm{x})))=y \lor\\ f_\theta(\mathcal{S}(\mathcal{P}(\bm{x})))\neq f_\theta(\mathcal{P}(\bm{x}))) / \text{\#}(True)$
\end{itemize}

\subsection{Attack Details}
\label{sec:attack_detail}
\paragraph{BadNets.} A $3\times 3$ grid is applied on the bottom right corner of each poisoned image.
\paragraph{Blend.} We blend images with Hello Kitty pattern under blend ratio $\alpha=0.2$. We also tried the random noise pattern, which is also commonly used in Blend attack. DBD fails under this setting, but other attacks work effectively.
\paragraph{Dynamic.} We use the pre-trained generator provided by the authors\footnote{https://github.com/VinAIResearch/input-aware-backdoor-attack-release} to create trigger pattern for each sample.
\paragraph{WaNet.} The original paper assumes that attackers has full control over the training process. We convert it into a poisoning-based method following the DBD paper. On CIFAR-10, we keep the original setting where control grid size $k=0.4$, warping strength $s=0.5$, and the noise rate $\rho_n=0.2$. We remove the noise mode on tiny-ImageNet to maintain the attack effectiveness of WaNet and set $k=8, s=1$.
\paragraph{CL.} We use the adversarial perturbation method with an $l_{\infty}$-norm bound and maximum perturbation size $\epsilon=32$. A grid is applied to training samples after perturbation. We trigger the backdoor with the grid during inference.

We present a few examples of the attacks mentioned above in \cref{fig:attack_examples}. The attacks are tested on CIFAR-10 and tiny-ImageNet. We train models on the benchmarks for 100 epochs with three data augmentations: random crop (padding size 4), horizontal flipping (with probability 0.5), and cutout ($3\times3$ square with random position). 
The initial learning rate is set to 0.1 (0.3 under ResNet-50) and decays with the cosine decay schedule.
We set weight decay to 1e-4 (5e-4 under tiny-ImageNet or ResNet-50) and batch size to 64 (128 for tiny-ImageNet).

\begin{figure}[t!]
    \centering
    \includegraphics[width=1.0\linewidth]{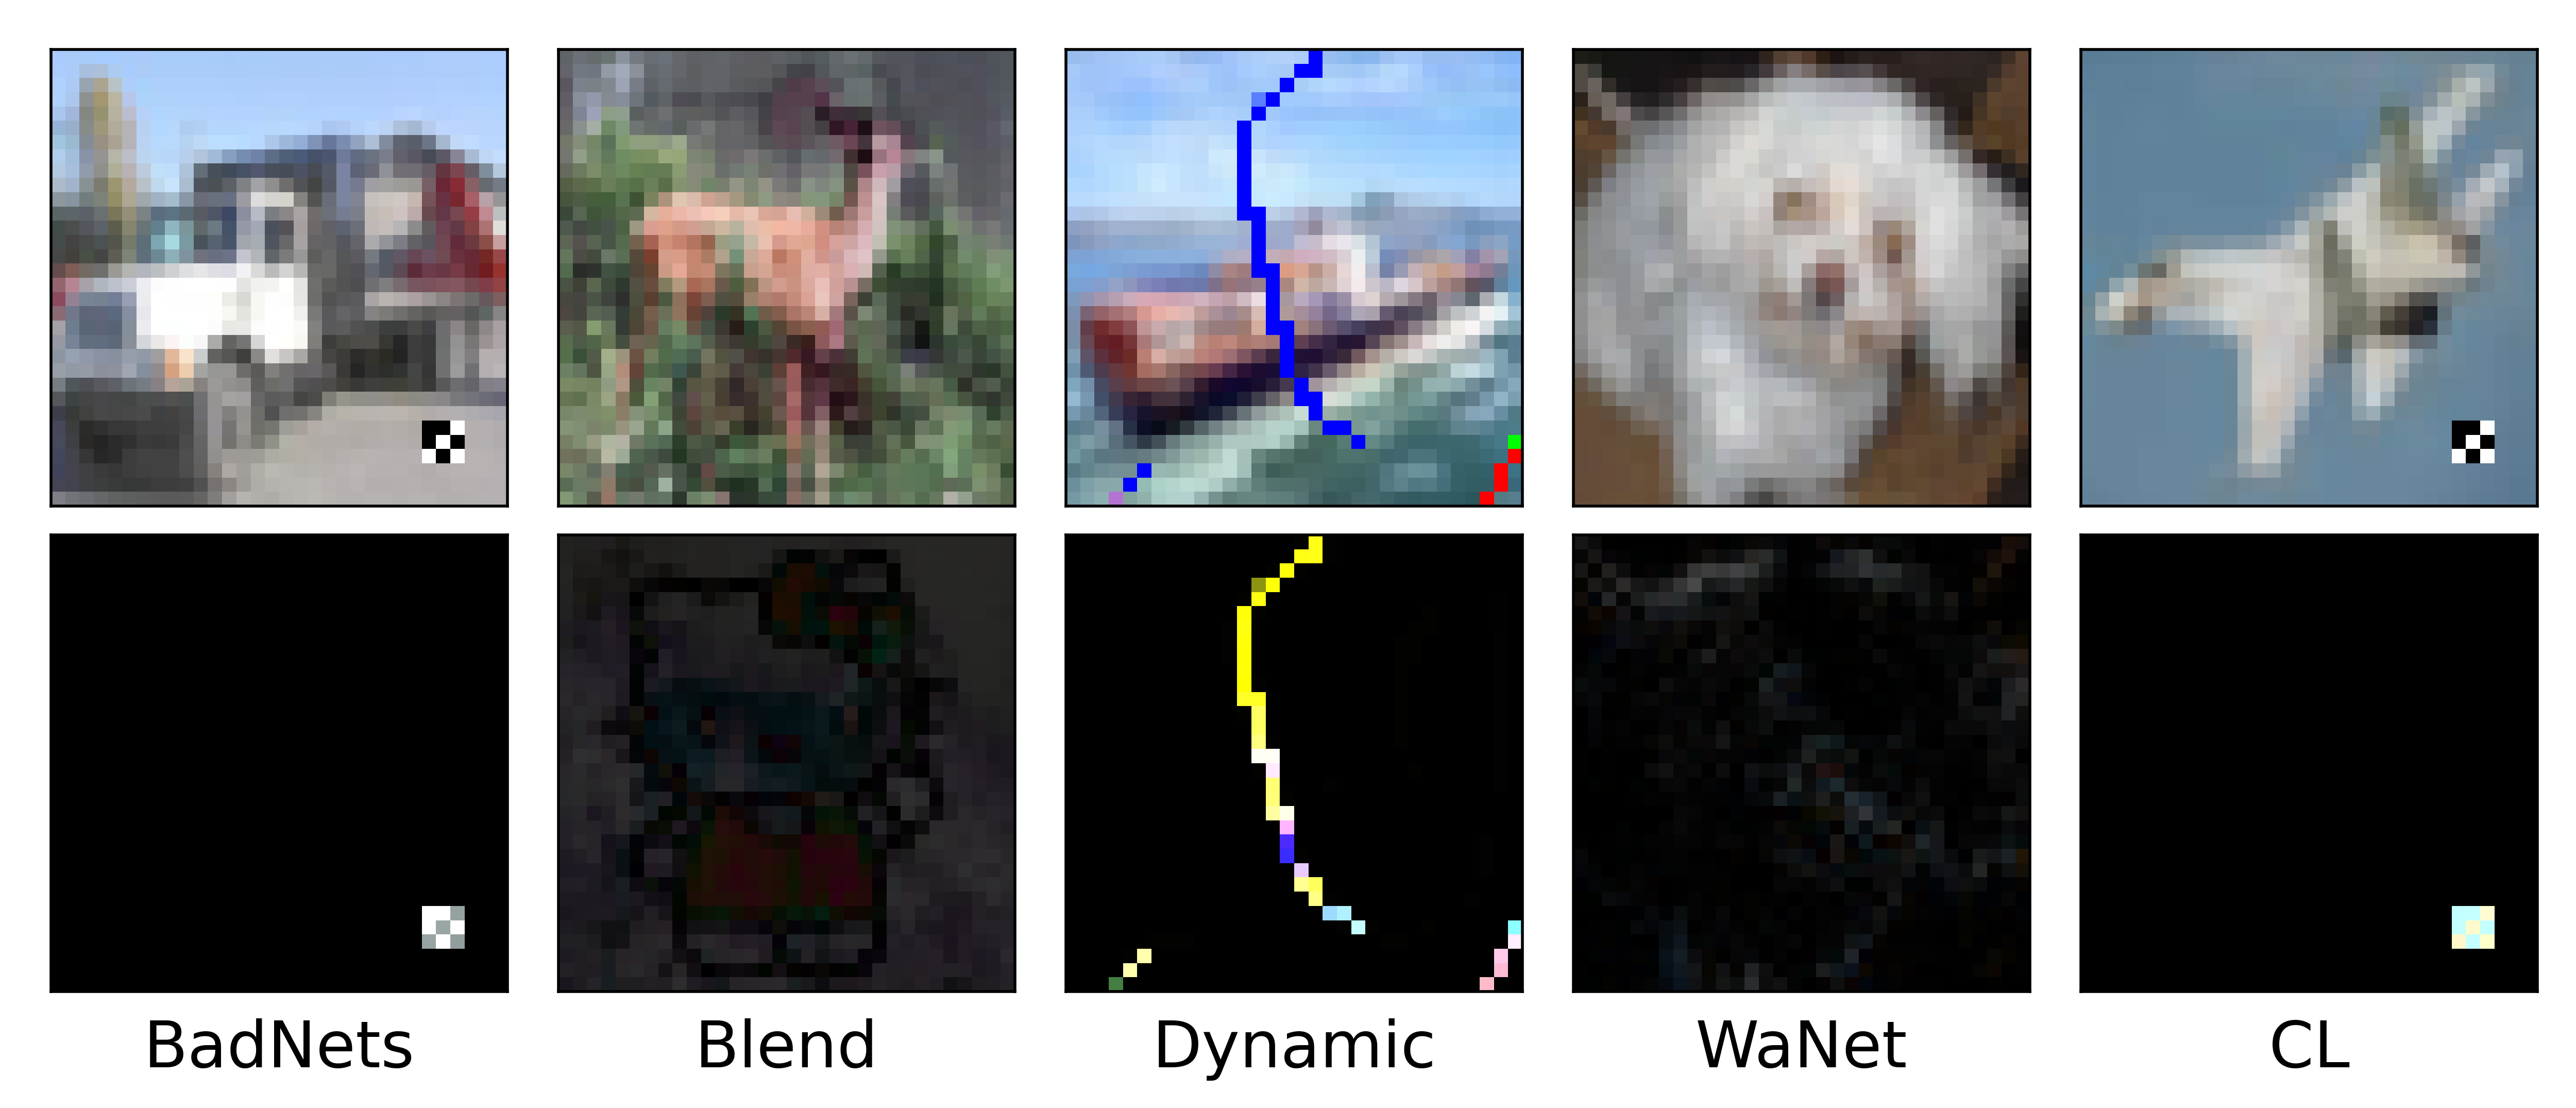}
    \caption{Poisoned images under different attacks (top) and the corresponding magnified ($\times2$) residual maps (bottom)}.
    \label{fig:attack_examples} 
\end{figure}

\subsection{Details of Defense Baselines}
\label{sec:defense_baseline}
\paragraph{NAD.} 
We modified the open-sourced implementation\footnote{https://github.com/bboylyg/NAD} to experiment on ResNet-18 and ResNet-50. 
The NAD loss is calculated over
the last residual group. 
5\% of the clean training data constitutes a local benign set as assumed in the original paper. 
We finetune a teacher model on the benign set, and then finetune a student model with cross-entropy and NAD loss: $\mathcal{L}_{ce}+\beta\mathcal{L}_{NAD}$.
The performance of NAD is sensitive to $\beta$, which typically brings a trade-off between CA and ASR as shown in \cref{tab:nad_beta}. $\beta=500$ is finally chosen for the main results as we attach importance to CA under comparable ASR.

\begin{table}[t!]
    \centering
    \setlength\tabcolsep{3.8pt}
    
    \begin{tabular}{c|cc|cc|cc}
    \toprule[1.2pt]
        $\beta$ & \multicolumn{2}{c|}{\textbf{500}} & \multicolumn{2}{c|}{\textbf{1000}} & \multicolumn{2}{c}{\textbf{1500}}\\\hline
        \textbf{Attack $\downarrow$} & ASR & CA & ASR & CA & ASR & CA  \\\hline
        \textbf{BadNets} & 4.47 & 90.39 & 2.04 & 89.09 & 1.78 & 88.10 \\
        \textbf{Blend} & 0.78 & 90.48 & 1.22 & 89.29 & 0.79 & 88.42 \\
        \textbf{Dynamic} & 10.63 & 90.08 & 10.28 & 89.11 & 6.49 & 89.00 \\
        \textbf{WaNet} & 2.74 & 89.94 & 1.31 & 88.52 & 1.08 & 87.33 \\
        \textbf{CL} & 6.96 & 89.42 & 4.63 & 88.97 & 3.38 & 88.57 \\
    \bottomrule[1.2pt]
    \end{tabular}
    \caption{Defense effectiveness (\%) of NAD under different $\beta$.}
    \label{tab:nad_beta}
\end{table}

\paragraph{ABL.}
We follow the training pipeline in the open-sourced code \footnote{https://github.com/bboylyg/ABL\#anti-backdoor-learning}. 
No data augmentation is adopted in the isolation and unlearning stage.
Note that an additional fine-tuning stage is added before backdoor unlearning to improve clean accuracy for fair comparison. 
ABL can reduce ASR to a negligable level in some cases, but we find the method sometimes unstable during unlearning. CA drops significantly even under a small learning rate. Therefore, we adopt an early stop strategy when we find CA drops below an acceptable level.

\paragraph{DBD.}
DBD achieves impressive performance under several attacks.
In the main experiments, we only modify the data loading and poisoning part of the open-sourced implementation\footnote{https://github.com/SCLBD/DBD} to fit our data format and keep other components unchanged.
Their results can be reproduced as presented in the paper when following the original attack settings.
However, we find two weaknesses of DBD in our explorations, hence providing comparisons with the method separately from other methods:
\begin{itemize}
\setlength\itemsep{-0.4em}
    \item The original implementation does not poison samples from the target class. When this constraint is removed, we find that a large number of poisoned samples from the target class are recognized as high-credible samples. They suffice to create a backdoor in a way similar to label-consistent attacks and enhance it by introducing more poisoned samples in the semi-supervised learning stage. In our experiments, ASR rises to 100\% and 4.06\% under BadNets and WaNet, respectively after removing the constraint.
    \item DBD relies on the assumption that representations of poisoned samples are not clustered after the self-supervised learning stage. However, we find that the assumption does not hold under Dynamic attack and random-noise-based Blend attack, because these attacks leaves explicit backdoor patterns in images even under strong data augmentation. In this case, poisoned samples will be considered as ``high-credible".
\end{itemize}

\subsection{Details of Our Method}
NAB poisons the training data and stamps every input in the test stage. Since the training pipeline is not modified, we simply follow the training settings in \cref{sec:attack_detail}. Here we provide more details about the detection and relabeling strategies adopted. Note that we use the same self-supervised learning model for DBD, LN and NC. Please refer to the DBD paper for computational cost.

\paragraph{Backdoor Detection.} The detection strategies we tried are modified from existing methods. They are probably not the best methods available and have limitations in some aspects, but are simple and strong enough to demonstrate the effectiveness of NAB. 
LGA is proposed as the backdoor isolation method in ABL. It is based on the observation that training losses of poisoned samples drop faster than clean samples. This assumption makes it vulnerable to some attacks like WaNet, which introduces a noise mode to make the backdoor harder to learn. We follow the original settings but increase the number of training epochs. 
LN is modified from the second stage of DBD. It aims at separating poisoned and clean samples using label-noise learning. We freeze the feature extractor and train the classifier with symmetric cross-entropy. Samples with the highest losses are suspected and isolated. LN also inherits the second weakness of DBD in \cref{sec:defense_baseline}. 
SPECTRE is a detection-based defense method targeting all-to-one attack. We re-implement it to function as a component of NAB. The modified SPECTRE identifies the target class according to the average QUE score. Then a specified number of samples in the target class with the highest QUE scores are detected as poisoned.

\paragraph{Pseudo Labels.} 
We introduced two simple pseudo label generation methods for relabeling. For VD, we adopt the same set of verified data as the one in the defense baseline NAD. We train a model on the verified data and predict pseudo labels on the poisoned training set. In NC, we remove a set of suspected data (20\% of the training set) to reduce the influence of poisoned samples whose representations are to some extent affected by the backdoor. 
The suspected data can be obtained by simply increasing the detection rate $\mu$ to $0.2$.
For each image-label pair $(\bm{x}, y)$ in the remaining data $\mathcal{D}_r$, we obtain representation of the image using the feature encoder $g$ of the SSL pre-trained model and compute class centers $c_i = \frac{1}{|\mathcal{D}_{r}^{(i)}|}\sum_{\bm{x}\in \mathcal{D}_{r}^{(i)}} g(\bm{x})$, where $\mathcal{D}_{r}^{(i)} = \{\bm{x}|(\bm{x},y)\in \mathcal{D}_r\land y=i\}$. 
Pseudo label $y'$ is assigned according to the nearest center for each sample: 
\begin{equation}
    y' = \argmin_i(\lVert g(\bm{x}) - c_i  \rVert_2)
\end{equation}

\section{Additional Experiments and Analyses}
Some of our experiments and analyses are not presented in the paper due to page limitation. We display them here for reference.

\begin{table}[t!]
    \centering
    \setlength\tabcolsep{2pt}
    
    \begin{tabular}{c|ccc|cccc}
    \toprule[1.2pt]
        {\textbf{Defense}} & \textbf{NAD} & \textbf{ABL} & \textbf{NAB} & \multicolumn{4}{c}{\textbf{NAB + filtering}} \\\hline
        \textbf{Attack $\downarrow$} & \multicolumn{3}{c|}{BA} & C-REJ & PSR & B-REJ & DSR  \\\hline
        {BadNets} & 88.24 & 92.62 & 76.40 & 2.66 & 92.91 & 99.75 & 100 \\
        {Blend} & 82.28 & 88.16 & 74.62 & 1.01 & 93.98 & 97.76 & 99.89 \\
        {Dynamic} & 72.95 & 87.68 & 67.14 & 1.09 & 93.92 & 97.05 & 99.88 \\
        {WaNet} & 87.35 & 87.33 & 82.07 & 5.40 & 90.32 & 90.04 & 99.48 \\
        {CL} & 87.69 & 87.85 & 83.35 & 4.67 & 90.99 & 87.62 & 99.57 \\\hline
        \textbf{Average} & 83.70 & 88.73 & 76.72 & 2.97 & 92.42 & 94.44 & 99.76 \\
    \bottomrule[1.2pt]
    \end{tabular}
    \caption{Backdoor accuracy (\%) and effectiveness (\%) of data filtering on ResNet-50.}
    \label{tab:filter_r50}
\end{table}

\subsection{Data Filtering on ResNet-50}
We present the effectiveness of data filtering on ResNet-50 in \cref{tab:filter_r50}. The results are consistent with conclusions in the paper.

\subsection{Backdoor Detection and Pseudo Label Quality}
We state in Sec. 4.4 that accuracy cannot fully reflect the quality of backdoor detection and pseudo label generation. In this section we give more intuition of this idea.

\paragraph{Pseudo Label.} 
As shown in \cref{fig:pseudo_label_matrix}, when misclassification happens, a model is more likely to predict a class in some way similar to the authentic one. For example, 39.6\% of the misclassified samples of automobile are predicted to truck, while only 2.4\% are predicted to bird. This property cannot be obtained by randomly generated pseudo labels.

\paragraph{Backdoor Detection.} 
In the experiments, we find that different backdoor detection methods might bring different defense effectiveness even under the same accuracy. 
We attribute this phenomenon partly to \textit{detection bias}, which means that a detection method has a preference for detecting poisoned samples with some explicit patterns. 
For example, LGA prefers to isolate images whose losses drop faster, while LN detect samples with higher losses in label-noise learning. 
When the samples share a unique feature $\alpha$ which is not the backdoor trigger and uncommon outside the detected set, the model might inject a non-adversarial targeting poisoned samples with feature $\alpha$. This will hamper the defense performance of NAB.
LGA works well in our experiments, but we find LN suffers from detection bias in rare cases as shown in \cref{fig:detection_bias}. 
ASR decreases to a negligible level in early training epochs, but the defense effectiveness quickly drops as the model learns to relate the non-adversarial backdoor to some specific features other than trigger pattern.

\begin{figure}[t!]
    \centering
    \includegraphics[width=0.9\linewidth]
    {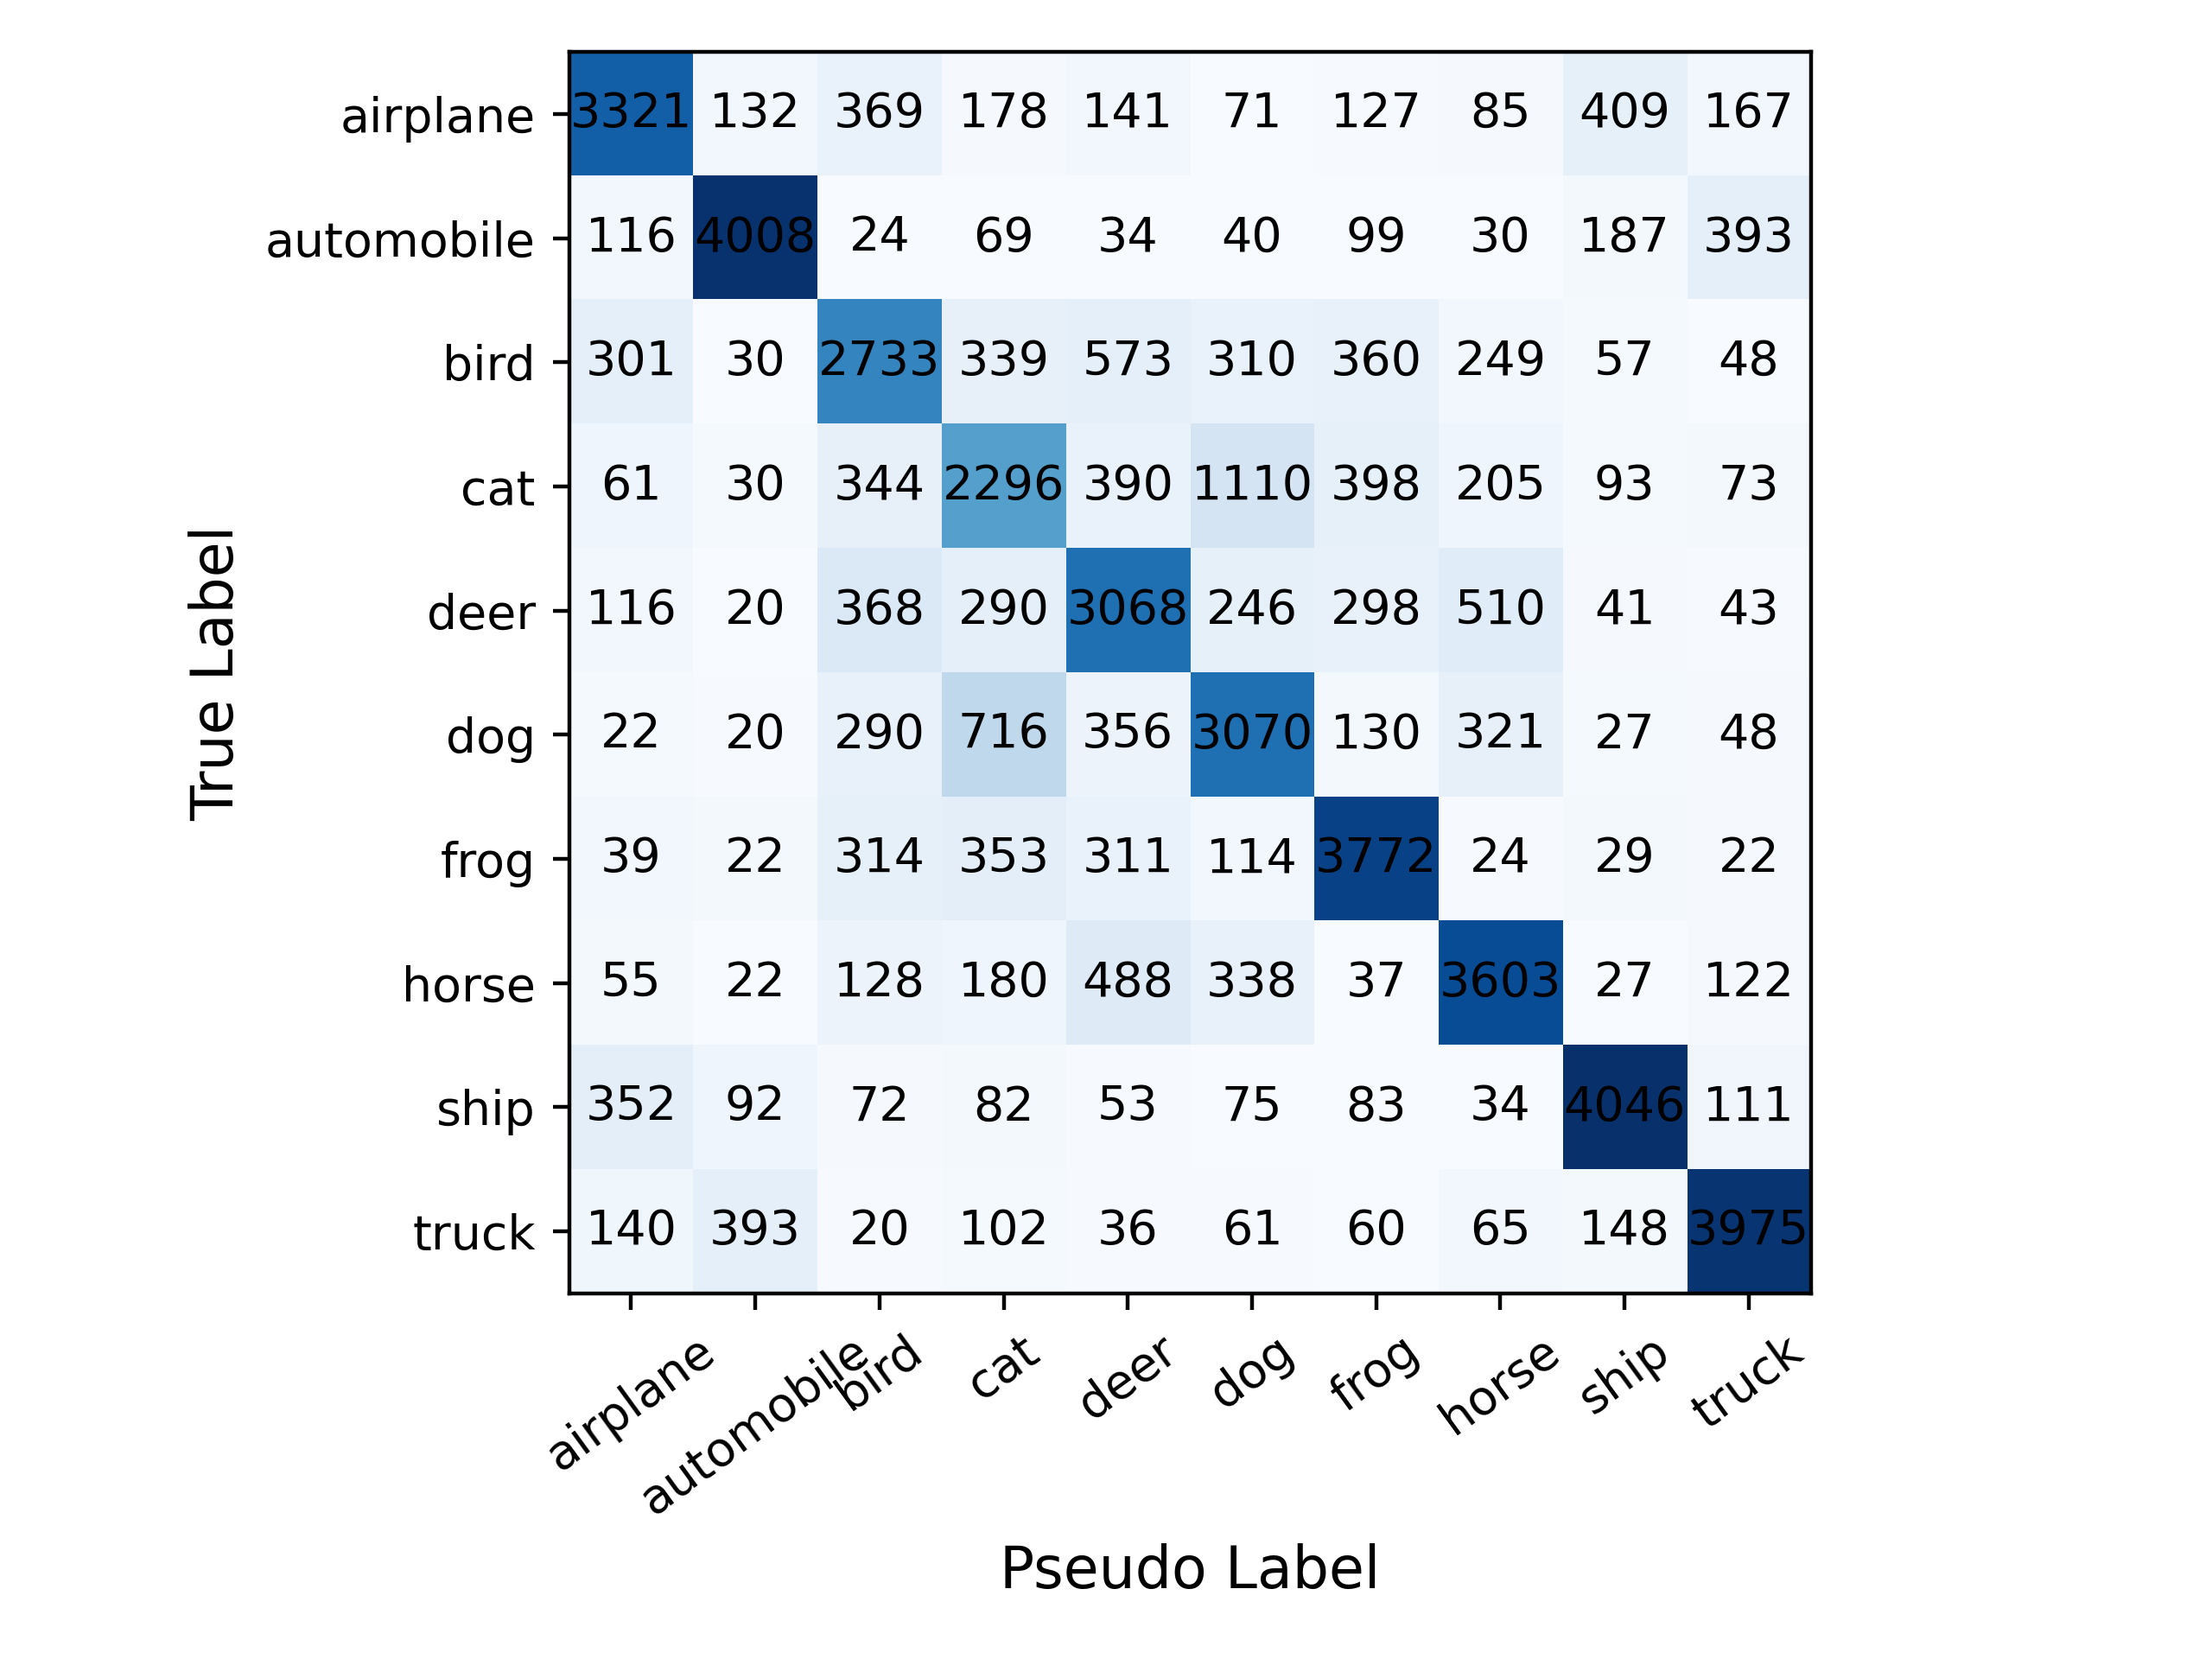}
    \caption{Details of pseudo labels generated by VD under BadNets attack on CIFAR-10.}
    \label{fig:pseudo_label_matrix} 
\end{figure}

\begin{figure}[t!]
    \centering
    \includegraphics[width=1.0\linewidth]
    {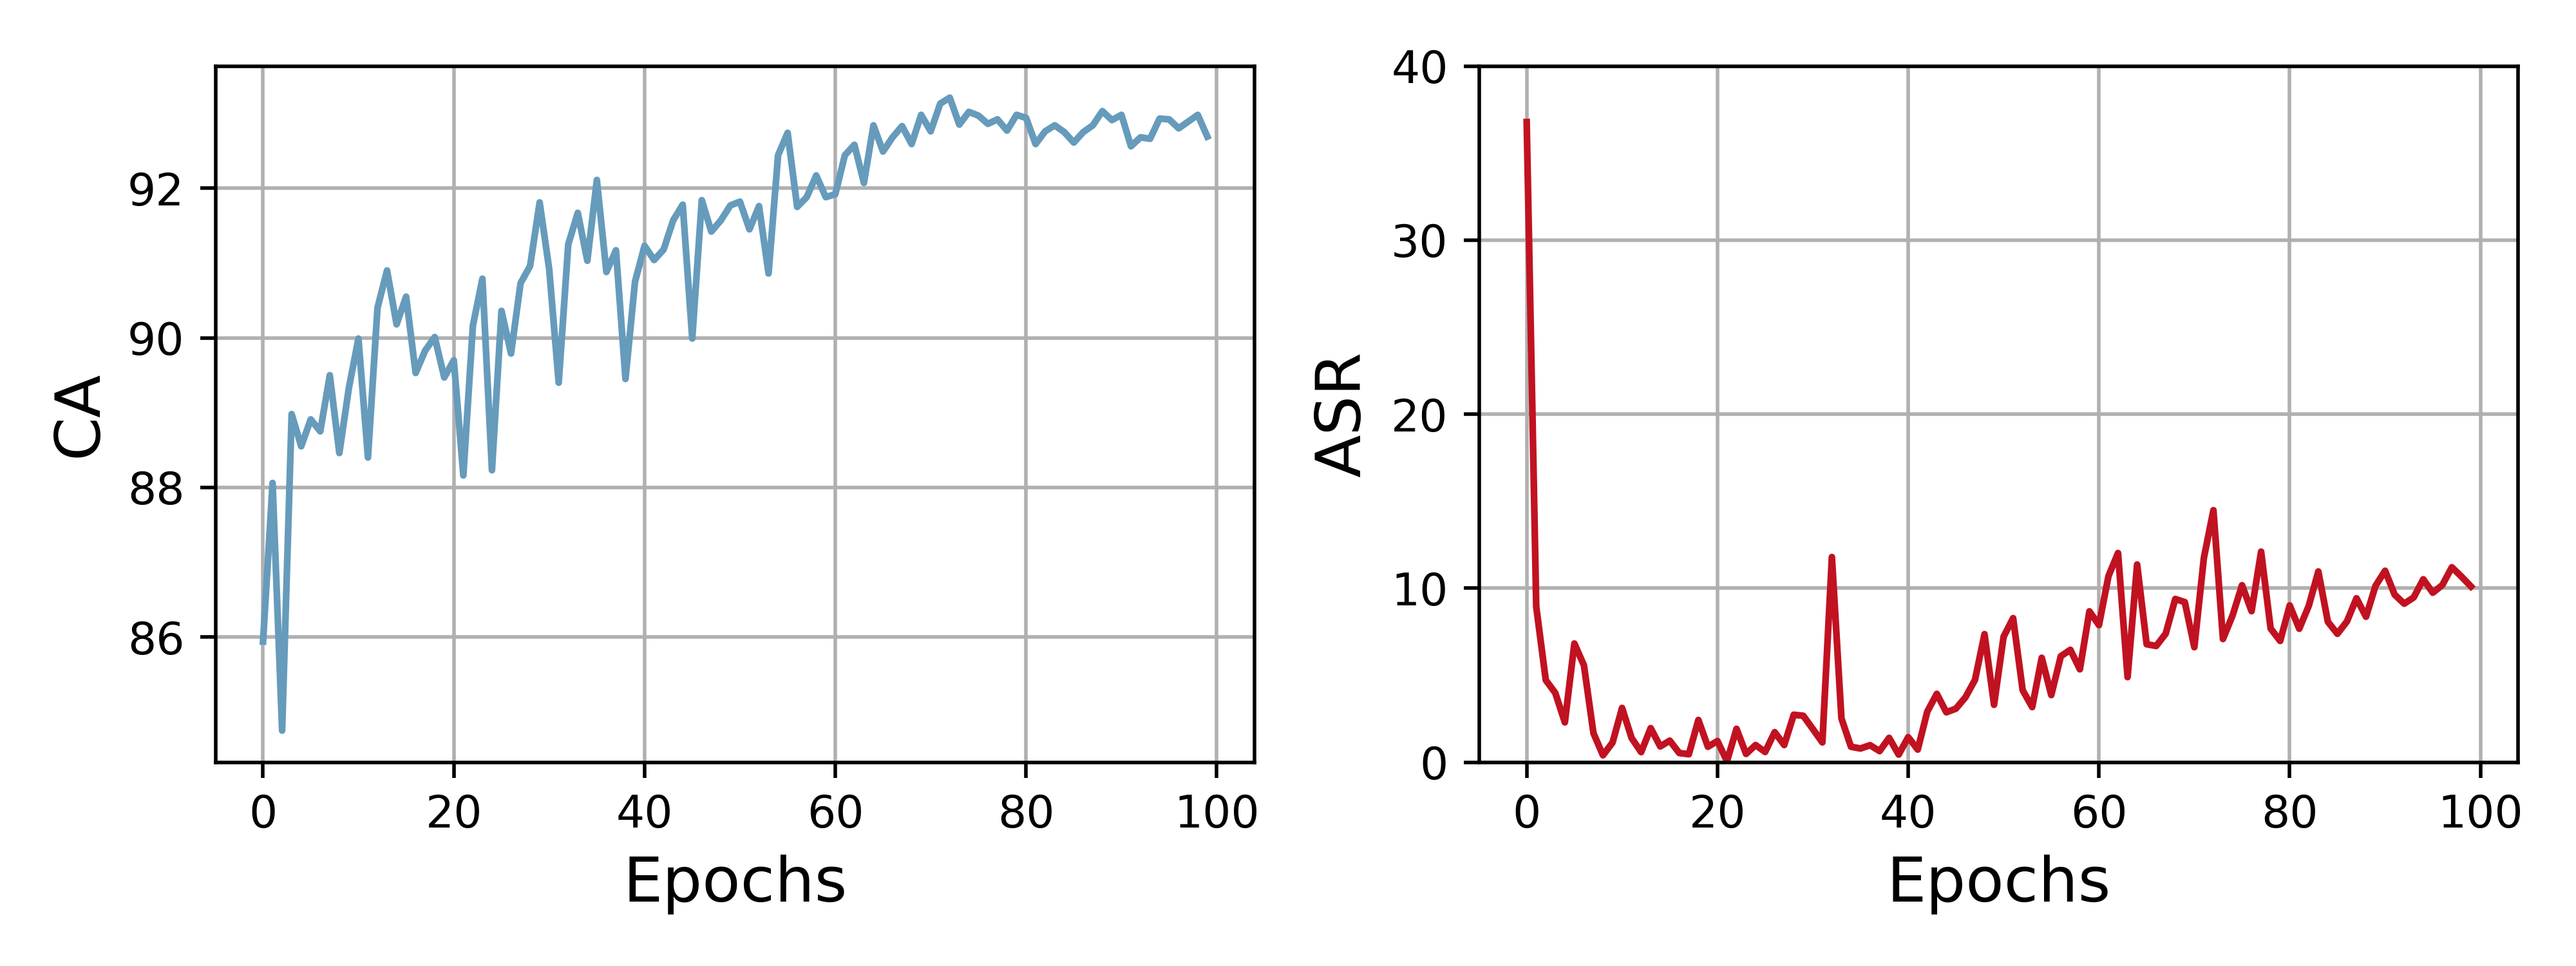}
    \caption{Illustration of detection bias. The experiment is conducted under Blend attack on CIFAR-10, using an SSL pre-trained ResNet-18 and LN detected samples.}
    \label{fig:detection_bias} 
\end{figure}

\begin{figure}[t!]
    \centering
    \includegraphics[width=1.0\linewidth]
    {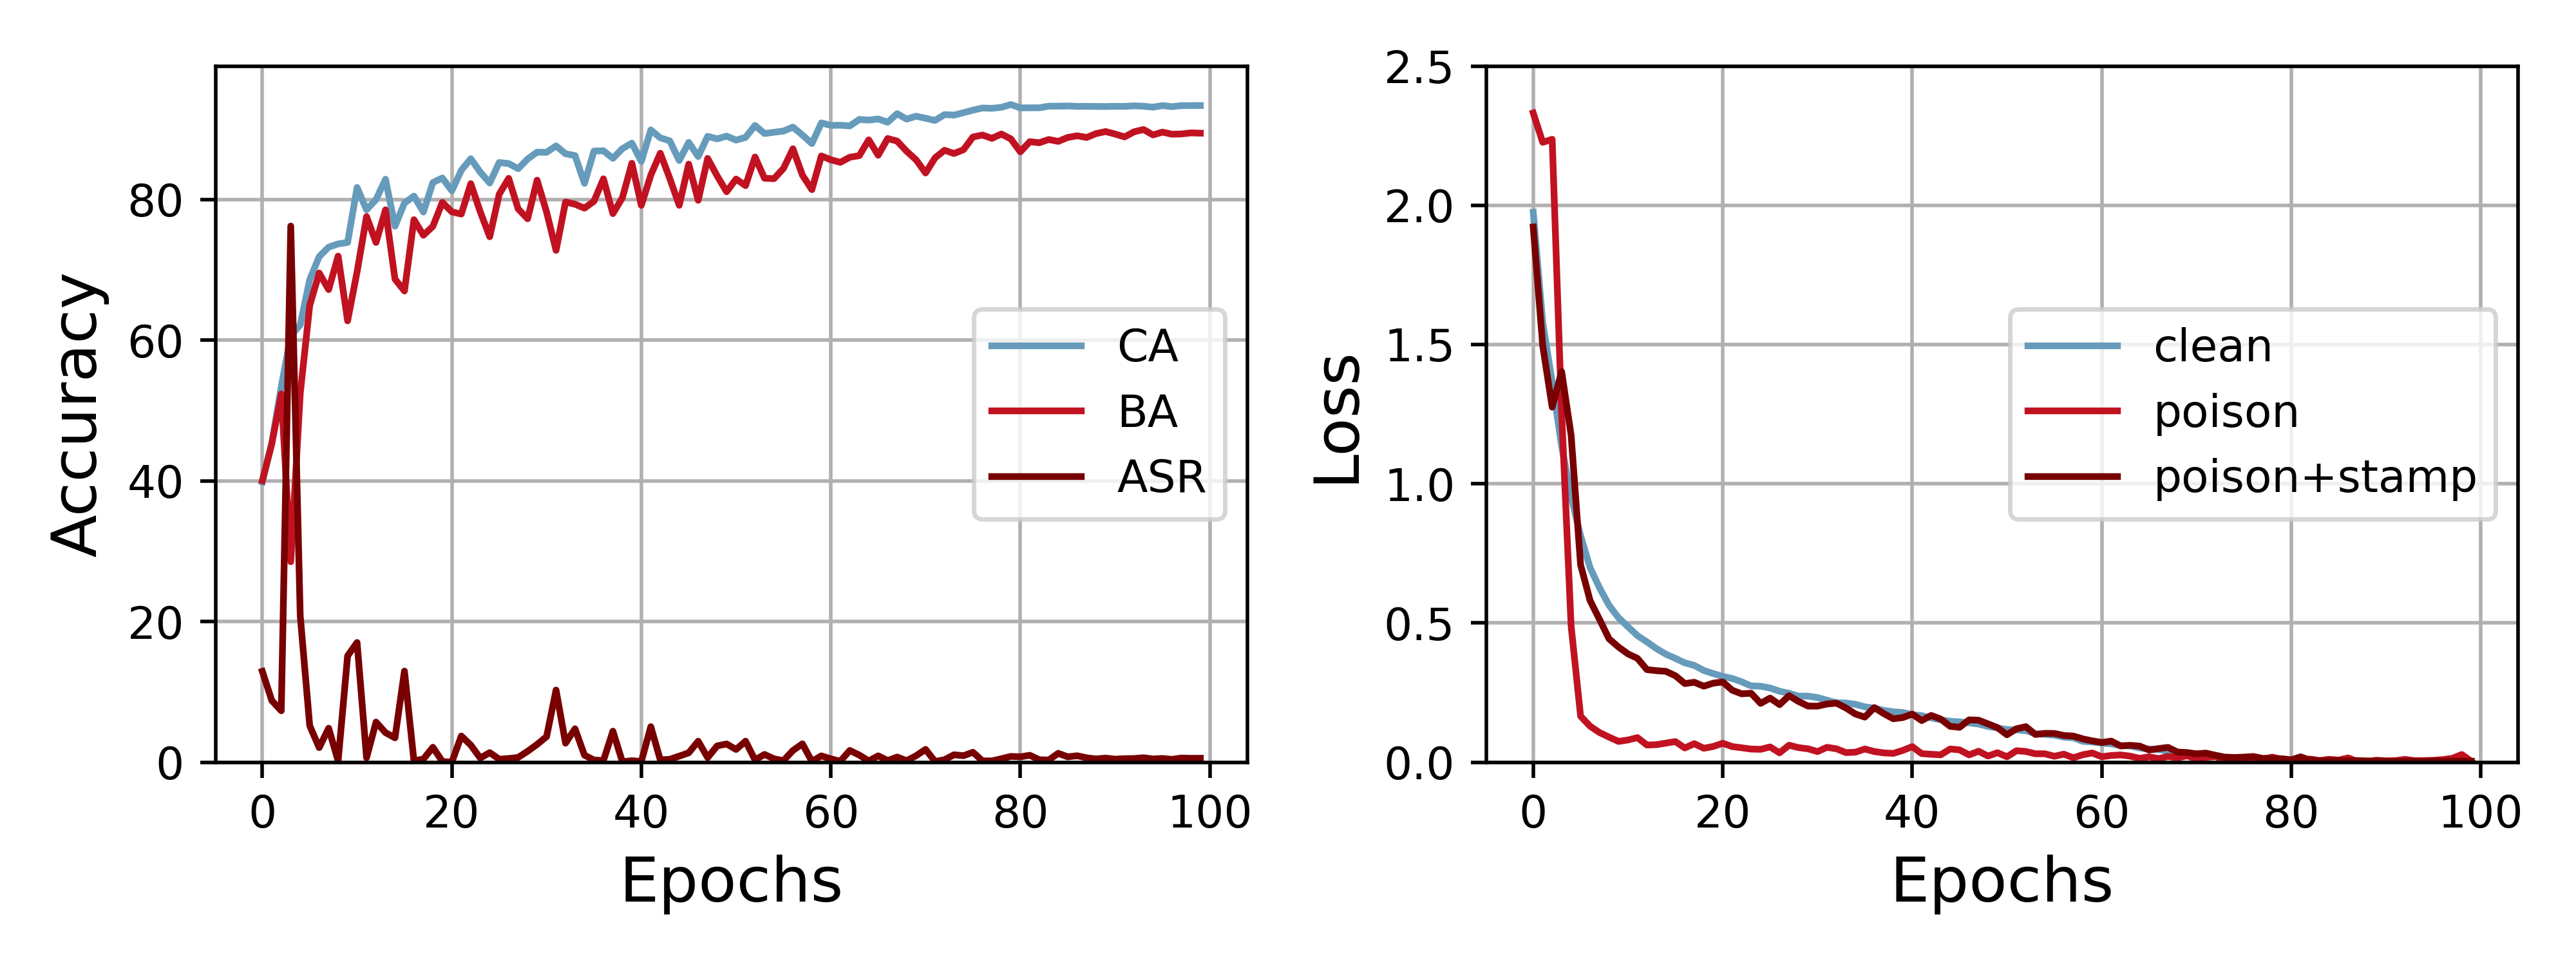}
    \caption{Illustration of training process using NAB under BadNets attack. LGA and NC are adopted for detection and relabeling, respectively.}
    \label{fig:process} 
\end{figure}

\subsection{Training Process Visualization}
NAB is implemented during data pre-processing and does not modify the training pipeline, so we dismissed details about the training process in the paper. 
Here we display how the non-adversarial backdoor is injected during training. 
As shown in \cref{fig:process}, our defense takes effect in the early epochs.
The losses of poisoned samples drop fast at the beginning, increasing ASR to a high level.
However, the non-adversarial backdoor is also learned after a few epochs and suppresses the adversarial backdoor effectively.

\begin{figure}[t!]
    \centering
    \setlength{\abovecaptionskip}{0.2em}
    \includegraphics[width=1.0\linewidth]{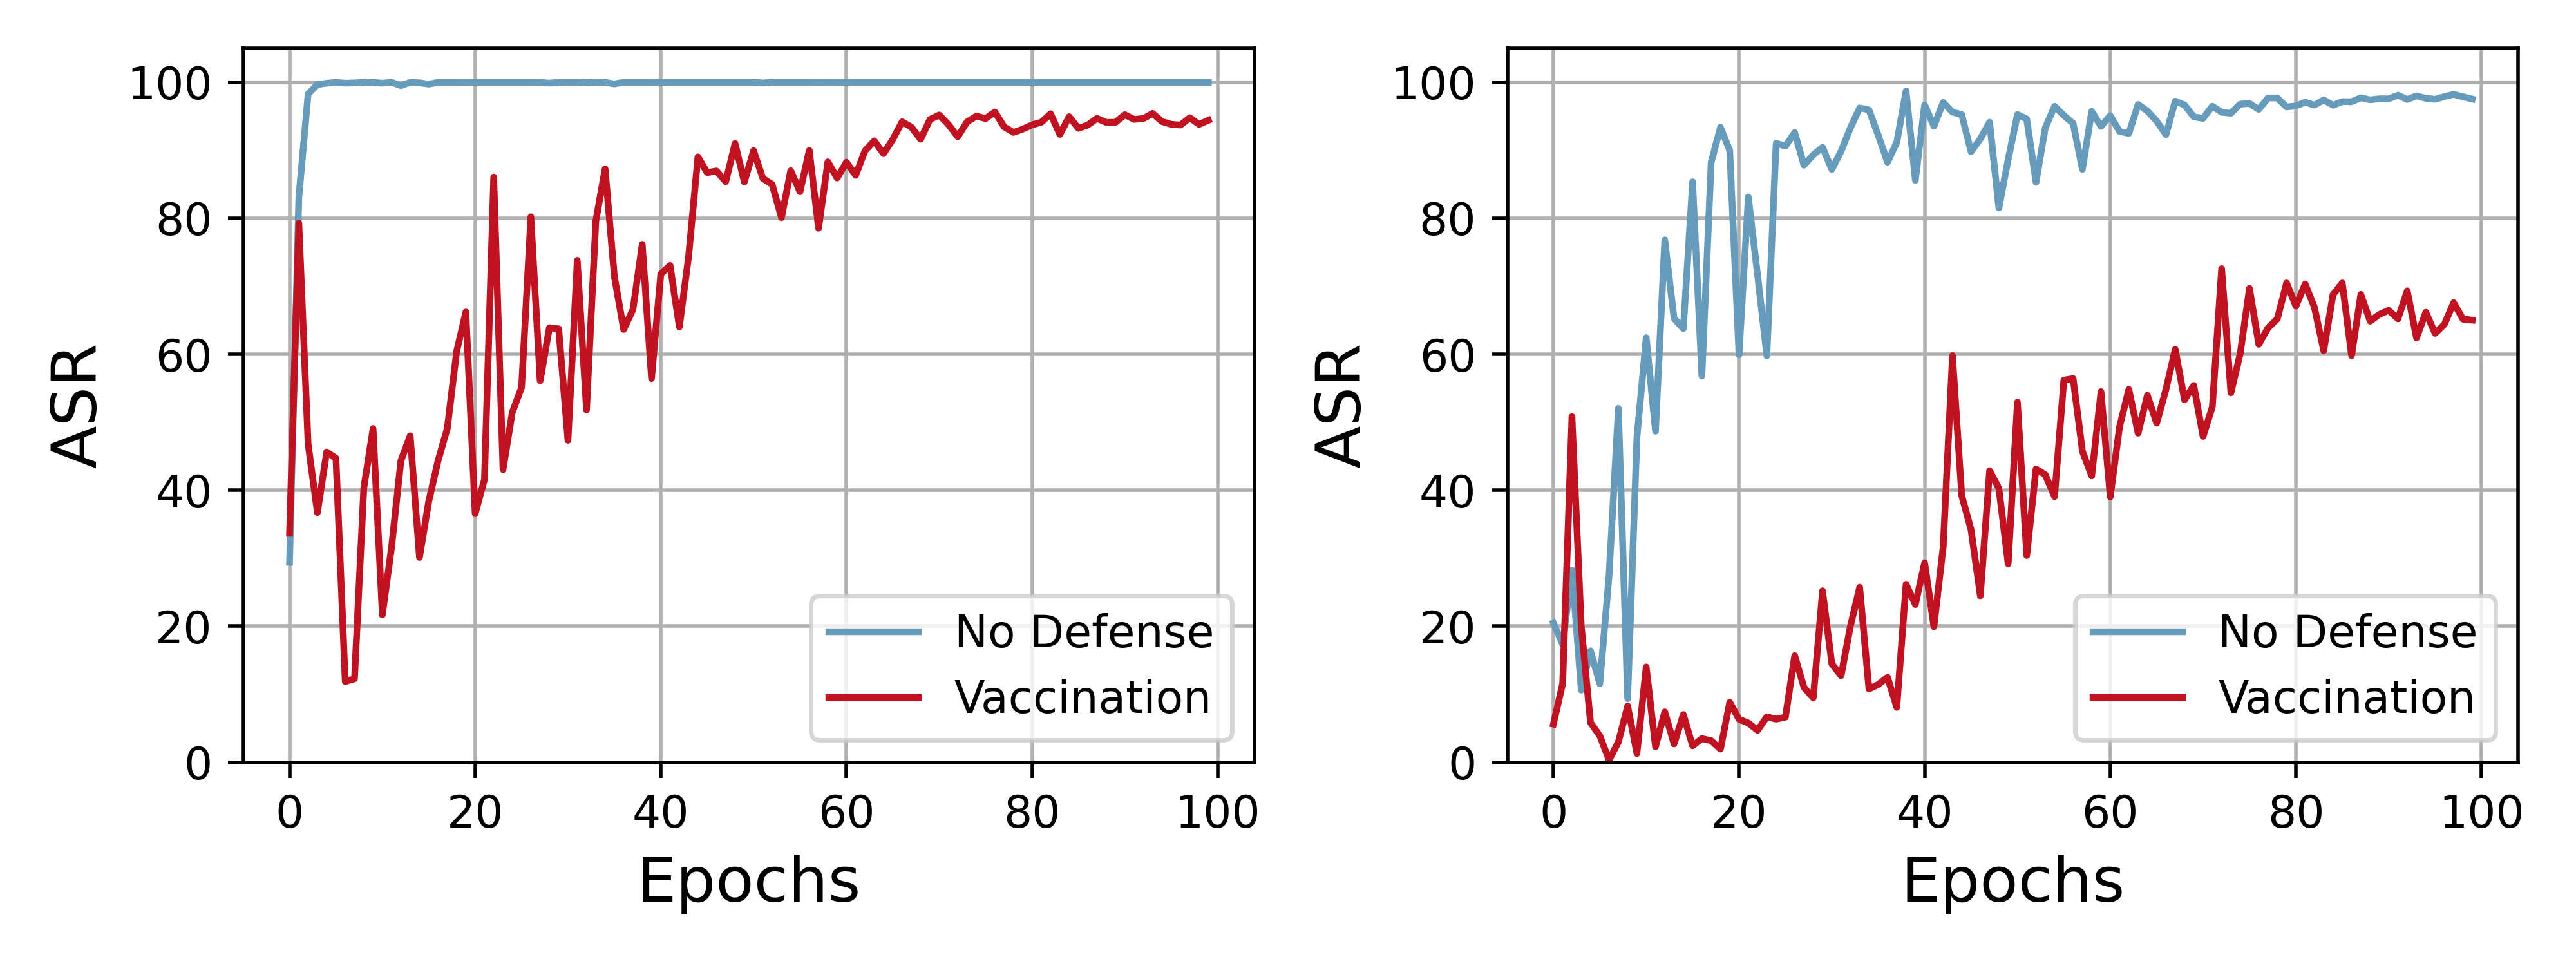}
    \caption{ASR (\%) of Blend attack (left) and WaNet attack (right) under no defense and backdoor vaccination. The defender implements BadNets attack and defend against it using NAB in backdoor vaccination.}
    \label{fig:vaccination} 
\end{figure}

\section{More Discussion on NAB}
\subsection{Backdoor Vaccination}
Compared with the simple data selection and relabeling steps in backdoor attack, it takes defenders more efforts to design and implement backdoor detection and pseudo label generation in NAB.
To free defenders from such trouble, we might need to reduce or totally mitigate the reliance on the two components.
In the paper we mentioned a few directions to achieve this goal, and backdoor vaccination is one of the promising ideas that we think is worthy of further exploration.

Backdoor vaccination is derived from the idea that the defense effectiveness of NAB under one attack might be generalized to other attacks.
If the generalization ability is strong enough, the defender can simply implement a backdoor attack and defend against it without being aware of the other attacks. Since we know which samples are poisoned and their original labels, we only need to select part of the poisoned samples and relabel them with the original labels.
A simple experiment is conducted to demonstrate the generalization ability. The defender is assumed to know the target class. We introduce a set of samples poisoned by BadNets and then process part of them with NAB. The set of data is merged with the original training set, which is poisoned by the attacker using another attack strategy (Blend and WaNet attack).  As shown in \cref{fig:vaccination}, backdoor vaccination can lower the attack success rate, especially in early epochs. The stealthier but somewaht weaker WaNet attack suffers more from the strategy. 
Backdoor vaccination is promising but so far not strong enough to become a defense strategy. We leave explorations along this direction as future work.

\subsection{Effectiveness under Adaptive Attack}
In some cases, attackers are aware of the defense strategy and adopt adaptive attacks to bypass it. 
We cannot find an easy attack strategy to nullify the non-adversarial backdoor, which is the core of our framework, but attackers can focus on the specific backdoor detection and poisoning strategies utilized and design adaptive attacks. For example, attackers can reduce detection accuracy or strengthen detection bias to make NAB less effective. Since the detection and poisoning strategies are replaceable and irrelevant to the core of our paper, we do not stress the topic here and leave it as a factor to consider when instantiating NAB.
